# Supplementary material for: Adapting Personalized Speech Enhancement for Low-Latency Audio-Visual Target-Speaker Extraction
Source: arXiv:2609.30631 source file (2026-09-24)
Supplement: Supplementary file 1 [file additional-human-results.tex]

% Numerical source: author-supplied.tex, adopted at the user's direction on 2026-09-11.
% Scores and confidence intervals are supplied values; not independently recalculated.
% Source-only additional results. Not included in the main manuscript.
% Numerical provenance is the author's supplied revision, not the earlier report.
% These values/intervals were retained at the user's explicit direction after review.

\begin{table}[t]
\caption{Additional supplied V+E--PVQE differences on meetings. Each entry is V+E minus PVQE with its supplied 95\% confidence interval. Values were adopted at the author's direction on 11 September 2026 and were not independently recalculated.}
\label{tab:additional-pvqe}
\centering
\fontsize{9}{10.2}\selectfont
\setlength{\tabcolsep}{5pt}
\renewcommand{\arraystretch}{1.08}
\begin{tabular}{@{}llr@{}}
\toprule
Dataset & Scale & \(\Delta\) vs PVQE [95\% CI]\\
\midrule
AMI & SIG & $-.11$ [$-.36$, .14]\\
 & BAK & +.08 [$-.10$, .26]\\
 & OVRL & $-.06$ [$-.24$, .12]\\
\midrule
MCoRec & SIG & +.24 [.00, .48]\\
 & BAK & +.10 [$-.08$, .28]\\
 & OVRL & +.17 [$-.01$, .35]\\
\bottomrule
\end{tabular}
\end{table}

\begin{table*}[t]
\caption{Additional supplied UniTalk human personalized P.835 results. Mean ratings are followed by V+E-minus-baseline differences and supplied 95\% confidence intervals. Values were adopted at the author's direction on 11 September 2026 and were not independently recalculated.}
\label{tab:additional-unitalk}
\centering
\fontsize{9}{10.2}\selectfont
\setlength{\tabcolsep}{8pt}
\renewcommand{\arraystretch}{1.08}
\begin{tabular}{@{}lrrr@{}}
\toprule
System / comparison & SIG & BAK & OVRL\\
\midrule
AVASE & 2.31 & 1.54 & 1.52\\
PVQE & \best{3.89} & \best{3.56} & \best{3.25}\\
V+E & 3.79 & 2.08 & 2.32\\
$\Delta$ vs AVASE & \best{+1.48 [1.22, 1.74]} & \best{+.54 [.36, .72]} & \best{+.80 [.62, .98]}\\
$\Delta$ vs PVQE & $-.10$ [$-.35$, .15] & \best{$-1.48$ [$-1.66$, $-1.30$]} & \best{$-.93$ [$-1.11$, $-.75$]}\\
\bottomrule
\end{tabular}
\end{table*}
