# Supplementary material for: Adapting Personalized Speech Enhancement for Low-Latency Audio-Visual Target-Speaker Extraction
Source: arXiv:2609.30631 source file (2026-09-24)
Supplement: Supplementary file 2 [file supplementary-training-comparison.tex]

% Source-only: moved from main paper to keep the selected-model tests together.
Training-data changes also affect preservation. From the same warm start, continuing on LRS3 alone instead of both corpora raises LRS3 SI-SNRi by 0.17 dB but lowers VoxCeleb2 SI-SNRi by 1.09 dB and increases its long suppression events from 23 to 203. Both continuations use the same architecture, optimizer, batch size, and 30-epoch schedule. Both warm starts have seen both corpora. With one run per recipe and different source reuse, this comparison supports retaining both corpora but does not isolate a causal effect of diversity.
